# Supplementary material for: Multilingual CheckList: Generation and Evaluation
Source: arXiv:2203.12865 source file (2022-10-12)
Supplement: Supplementary file 1 [file 0_appendix_kk.tex]

% This must be in the first 5 lines to tell arXiv to use pdfLaTeX, which is strongly recommended.
\pdfoutput=1
% In particular, the hyperref package requires pdfLaTeX in order to break URLs across lines.

\documentclass[11pt]{article}

% Remove the "review" option to generate the final version.
\usepackage[review]{acl}

% Standard package includes
\usepackage{times}
\usepackage{latexsym}

% For proper rendering and hyphenation of words containing Latin characters (including in bib files)
\usepackage[T1]{fontenc}
\usepackage{titlesec}
\setlength{\belowcaptionskip}{-12pt}
% \setlength{\topmargin}{-5pt}
\setlength{\topskip}{-5pt}
\addtolength{\baselineskip}{-5mm}

% \titlespacing\section{-1pt}{-1pt}{-1pt}
% \titlespacing\subsection{-10pt}{-1pt}{-1pt}


%%% For language switching -- like babel, but for xelatex
% \usepackage{fontspec}
% \setromanfont{Times New Roman}
% \setsansfont{Times New Roman}
% \setmonofont{Courier New}

% \usepackage{polyglossia}
% \setmainlanguage{english}
% \setotherlanguages{hindi} %% or other languages

% \renewcommand{\foreignlanguage}[2]{
%     \begin{#1} 
%     #2 
%     \end{#1}
% }
% \newfontfamily\devanagarifont[Script=Devanagari]{Lohit Devanagari}

% For Vietnamese characters
% \usepackage[T5]{fontenc}
% See https://www.latex-project.org/help/documentation/encguide.pdf for other character sets

% This assumes your files are encoded as UTF8
\usepackage[utf8]{inputenc}

% This is not strictly necessary, and may be commented out,
% but it will improve the layout of the manuscript,
% and will typically save some space.
\usepackage{microtype}
\usepackage{graphicx}
\usepackage{multirow}
\usepackage{booktabs}
\usepackage{enumitem}
\usepackage{arydshln}
\usepackage{algorithm}
% \usepackage{algorithmic}
\usepackage{algpseudocode}
\usepackage{amsmath}
\usepackage[multiple]{footmisc}
\usepackage{amsfonts}

\renewcommand{\algorithmicrequire}{\textbf{Input:}}
\renewcommand{\algorithmicensure}{\textbf{Output:}}
\mathchardef\mhyphen="2D % Define a "math hyphen"

\newtheorem{lemma}{Lemma}[section]
\newtheorem{explanation}{Explanation}[section]


% If the title and author information does not fit in the area allocated, uncomment the following
%
%\setlength\titlebox{<dim>}
%
% and set <dim> to something 5cm or larger.

\title{Multilingual CheckList: Generation and Evaluation}

% Author information can be set in various styles:
% For several authors from the same institution:
% \author{Author 1 \and ... \and Author n \\
%         Address line \\ ... \\ Address line}
% if the names do not fit well on one line use
%         Author 1 \\ {\bf Author 2} \\ ... \\ {\bf Author n} \\
% For authors from different institutions:
% \author{Author 1 \\ Address line \\  ... \\ Address line
%         \And  ... \And
%         Author n \\ Address line \\ ... \\ Address line}
% To start a seperate ``row'' of authors use \AND, as in
% \author{Author 1 \\ Address line \\  ... \\ Address line
%         \AND
%         Author 2 \\ Address line \\ ... \\ Address line \And
%         Author 3 \\ Address line \\ ... \\ Address line}

\author{Karthikeyan K\textsuperscript{3}*, Shaily Bhatt\textsuperscript{1}*, Pankaj Singh\textsuperscript{1}, Somak Aditya\textsuperscript{4},\\\bf{Sandipan Dandapat\textsuperscript{2}, Sunayana Sitaram\textsuperscript{1}, Monojit Choudhury\textsuperscript{1}}
\\
\textsuperscript{1} Microsoft Research, Bengaluru, India
\\
\textsuperscript{2} Microsoft R\&D, Hyderabad, India
\\
\textsuperscript{3} Department of Computer Science, Duke University
\\
\textsuperscript{4} Department of CSE, IIT Kharagpur
\\
\texttt{karthikeyan.k@duke.edu, saditya@cse.iitkgp.ac.in,}
\\
\texttt{\{t-shbhatt,t-pasingh,sadandap,sunayana.sitaram,monojitc\}@microsoft.com}
        }


\begin{document}
	\maketitle


\appendix

\input{v2_shaily/app_1_tea_details}

\end{document}
