# Supplementary material for: Multilingual CheckList: Generation and Evaluation
Source: arXiv:2203.12865 source file (2022-10-12)
Supplement: Supplementary file 3 [file appendix.tex]

\input{amcg-appendix}

\section{Proofs}

\noindent{\textbf{Lemma 1:}} If a valid template $t$ generates a sentence $s_i$, and if the terminals $w_m (\in $ non-terminal $v_m$), is sub-string(s) of $t$ ($w$ can occur any number of times in $t$). Then the valid template, $t^{\prime}$, formed by replacing any subset of the $w_m$ in $t$, by $v_m$ (with appropriately named cardinal), also generates $s_i$.

\noindent{\textbf{Proof: }}  Let $t$ already contains the non-terminal $v_m$ up to an cardinal of $h -- v_m^0, v_{m}^1, v_{m}^2, ... v_{m}^{h} $, (if $t$ does not contain $v_m$, then $h=-1$). To generate $t^{\prime}$, we first replace all the $w_m$ with $v_{m}^{h+1}$, lets call this intermediate template as $t^{temp}$. Then the cardinals of $v_m$ in $t^{temp}$ are renamed to make it the valid template $t^{\prime}$. But we know that renaming the cardinals does not change the language generated by the template. Therefore, if $t^{temp}$ generates $s_i$ then $t^{\prime}$ also generates $s_i$. To generate $s_i$ from $t^(temp)$, first replace all the $v_m^(h+1)$ with $w_m$, this generates $t$. But we know that $t$ generates $s_i$, therefore  $t^{\prime}$ also generates $s_i$. 

\noindent{\textbf{Corollary 1:}} Every template $t_{ik} \in T_i$ generates the sentence $s_i$

\noindent{\textbf{Proof: }} Repeatedly apply lemma 1 whenever we add a new template to the existing $T_i$. Note that the initial $T_i$ contains only $s_i$ and it can generate $s_i$. 

% \pagebreak



\noindent{\textbf{Lemma 2:}} If a valid template, $t$ generates $s_i$ using only the first $N$ elements from the list of $\langle$ terminal, non-terminal $\rangle$ tuples $L$, then $t \in T_i$ after $N^{th}$ iteration, i.e. after seeing the $N^{th}$ element of $L$ in the iteration.


\noindent \textbf{proof:} 

Let $t$ contain the $r$ distinct non-terminals, call them, $v_{a1}, v_{a2}, ... v_{ar}$ (note that $v_{ai}$ and $v_{aj}$ can be same non-terminal with different cardinals). Lets denote the non-cardinal form of a non-terminal $v_{ai}$ as $v_{ai}^{\prime}$, i.e. if $v_{ai} = v_m^h$ then $v_{ai}^{\prime} = v_m$. To generate $s_i$, $t$ has to use some mapping from non-terminal to terminal, $\forall ai, v_{ai} \rightarrow w_{ai}$, such that $(v_{ai}^{\prime}, w_{ai})$ belongs the first $N$ elements of list $L$. Further, by definition of a valid template in restricted grammar, $if v_{ai}^{\prime} = v_{aj}^{\prime}, and , i \neq j, then,  w_{ai} \neq w_{aj} $. Therefore all the tuples,  $(v_{ai}^{\prime}, w_{ai} )$ are distinct. Without loss of generality, in the list $L$, assume that $(v_{ai}^{\prime}, w_{ai} )$ comes earlier than before $(v_{aj}^{\prime}, w_{aj} )$ if $i < j$. 

We will prove the lemma by induction, assume that every valid template $t$ that has less than $r$ non-terminals and that generates $s_i$ using only the first $n$ elements of list $L$, belongs to $T_i$ after the $n^{th}$ iteration. 

\textbf{Base Case:} Let $t$ be a template that generates $s_i$. If $t$ contains $0$ non-terminals, then the only possible $t = s_i$ and $t\in T_i$ at $0^{th}$ iteration and every after iteration. 

Let $(v_{ar}, w_{ar})$ be the $n^{th}$ tuple in $L$. Replace {\em{all}} the $v_{ar}$ in $t$ with $w_{ar}$, call the new template $t^{temp}$. Rename the cardinals of non-terminals in $t^{temp}$ to make it a valid template, call it $t^{\prime}$. Note that $t^{\prime}$ contains less than $r$ non-terminals and generates $s_i$ using only the first $n-1$ elements of $L$, therefore, by induction assumption, $t^{\prime} \in T_i$ after the $(n-1)^{th}$ iteration. In the $n^{th}$ iteration, if $w_{ar}$ occurs once or more in $t^{\prime}$, we replace every subset of $w_{ar}$ with $v_{ar}^{\prime}$ with appropriate cardinal, to generate set of new templates. Among them, consider the following template, if a particular $w_r$ is a non-terminal in $t$ then replace it, otherwise leave it as $w_{ar}$, call this template $t^{new}$. Note that $t^{new}$ and $t$ are equivalent -- only the naming of cardinals of the non-terminal $v_{ar}^{\prime}$ are different. Therefore, by re-naming the cardinals of $t^{new}$, we get $t$ -- all the equivalent template will be mapped to the same template by renaming the cardinals according to our convention. Therefore, $t \in T_i$ after the $n^{th}$ iteration. 

hence, by induction, lemma 2 is proved. 

\noindent{\textbf{Corollary 2:}} Every valid template, that generates $s_i$ using only the given terminal, non-terminal (using only the list $L$) is present in the final $T_i$.


\noindent{\textbf{Lemma 3:}} Set $\hat{T}$ can generate every sentences in $S$

\noindent \textbf{proof:} To generate a sentence $s_i \in S$, consider any template, $t$, in the set $\hat{T} \cap T_i $ (not null). $t$ generates $s_i$ from corollary 1. 


\noindent{\textbf{Lemma 4:}} If a set $\hat{T}$ is the smallest set such that $\forall i, \hat{T} \bigcap T_i \neq \emptyset $, then $\hat{T}$ is the smallest set that generates every sentence in $S$ using only the given terminals and non-terminals. 

\noindent \textbf{proof:} Let $T^{\prime}$, such that, $|T^{\prime}| < |\hat{T}|$, be the smallest set of templates that generate every sentence in $S$ using only the given terminals and non-terminals. For every sentence $s_i$, we assumed that $T^{\prime} $ generates $s_i$. Therefore $T^{\prime} $ should have atleast one template that generates $s_i$ using only given terminals and non-terminals; call it $t$. From corollary 2, we know that $t \in T_i$. Therefore, for every $i$, $T^{\prime} \bigcap T_i \neq \emptyset $. But we know that $\hat{T}$ is the smallest set such that $\forall i, \hat{T} \bigcap T_i \neq \emptyset $, therefore $|T^{\prime}| \geq |\hat{T}|$, hence contradiction. 

\section{Examples}

We show some examples of how different aspects of translations (errors and syntactic divergences) may affect AMCG output in Table~\ref{app:examples}.
\begin{table*}[!ht]
\resizebox{\textwidth}{!}{%
\small
\begin{tabular}{|lllll|}
\hline
\multicolumn{1}{|l|}{\textbf{Source template}}                                                                                       & \multicolumn{1}{l|}{\textbf{Source Example}}                                                                  & \multicolumn{1}{l|}{\textbf{Target Examples}}                                                       & \multicolumn{1}{l|}{\textbf{Target Template}}                                                                                                       & \textbf{Comment}                                                         \\ \hline
\multicolumn{5}{|c|}{\textit{Translation Errors - Word Sense Disambiguation - Hindi}}                                                           \\ \hline
\multicolumn{1}{|l|}{\begin{tabular}[c]{@{}l@{}}The \{air\_noun\} is poor.\\ air\_noun = {[}'aircraft', 'service'{]}\end{tabular}}    & \multicolumn{1}{l|}{\begin{tabular}[c]{@{}l@{}}The aircraft is poor.\\ The service is poor.\end{tabular}}       & \multicolumn{1}{l|}{\begin{tabular}[c]{@{}l@{}}viman gareeb hai.\\ seva gareeb hai.\end{tabular}}     & \multicolumn{1}{l|}{\begin{tabular}[c]{@{}l@{}}\{key1\} gareeb hai.\\ key1 = {[}'viman', 'seva'{]}\end{tabular}}                                     & \begin{tabular}[c]{@{}l@{}}The word poor is translated to \\ ``gareeb''  which indicates poverty. \\ Similarly, the word "lame" is \\ translated to "langda" which \\ indicates physical disability.\end{tabular} \\ \hline

\multicolumn{5}{|c|}{\textit{Translation Errors - Word Sense Disambiguation - Gujarati}}        \\ \hline
\multicolumn{1}{|l|}{\begin{tabular}[c]{@{}l@{}}The \{air\_noun\} is poor.\\ air\_noun = {[}'aircraft', 'service'{]}\end{tabular}}    & \multicolumn{1}{l|}{\begin{tabular}[c]{@{}l@{}}The aircraft is poor.\\ The service is poor.\end{tabular}}       & \multicolumn{1}{l|}{\begin{tabular}[c]{@{}l@{}}viman gareeb che.\\ seva gareeb che.\end{tabular}}     & \multicolumn{1}{l|}{\begin{tabular}[c]{@{}l@{}}\{key1\} gareeb che.\\ key1 = {[}'viman', 'seva'{]}\end{tabular}}                                     & \begin{tabular}[c]{@{}l@{}}Similar to Hindi, \\the word {\em poor} is translated to \\ {\em ``gareeb''}  which indicates poverty. \\ Similarly, the word {\em lame} is \\ translated to {\em "langda"} which \\ indicates physical disability.\end{tabular} \\ \hline

\multicolumn{5}{|c|}{\textit{Syntactic Divergence - Hindi}}                                                                                                                    \\ \hline
\multicolumn{1}{|l|}{\begin{tabular}[c]{@{}l@{}}This is a good \{air\_noun\}.\\ air\_noun = {[}'aircraft', 'service'{]}\end{tabular}} & \multicolumn{1}{l|}{\begin{tabular}[c]{@{}l@{}}This is a good aircraft.\\ This is a good service.\end{tabular}} & \multicolumn{1}{l|}{\begin{tabular}[c]{@{}l@{}}yah acha viman hai.\\ yah achi seva hai.\end{tabular}} & \multicolumn{1}{l|}{\begin{tabular}[c]{@{}l@{}}yah \{key2\} \{key1\} hai.\\ key1 = {[}'viman', 'seva'{]}\\ key2 = {[}'acha', 'achi'{]}\end{tabular}} & \begin{tabular}[c]{@{}l@{}} In Hi, \textit{acha} is masculine form \\ of the adjective \textit{good} and that can \\ not be used with a feminine noun\\ i.e., \textit{seva} (service). The opposite \\ is also true. However, in the task \\ sentiment analysis, human-written \\ reviews may have similar noise and \\ such a Hence this does not affect \\ the usefulness of the template. 

\end{tabular}                    \\ \hline

\multicolumn{5}{|c|}{\textit{Syntactic Divergence - Gujarati}}                                                                                                                    \\ \hline
\multicolumn{1}{|l|}{\begin{tabular}[c]{@{}l@{}}This is a good \{air\_noun\}.\\ air\_noun = {[}'aircraft', 'service'{]}\end{tabular}} & \multicolumn{1}{l|}{\begin{tabular}[c]{@{}l@{}}This is a good aircraft.\\ This is a good service.\end{tabular}} & \multicolumn{1}{l|}{\begin{tabular}[c]{@{}l@{}}Aa saaru viman che.\\ Aa saari seva hai.\end{tabular}} & \multicolumn{1}{l|}{\begin{tabular}[c]{@{}l@{}}aa \{key2\} \{key1\} che.\\ key1 = {[}'viman', 'seva'{]}\\ key2 = {[}'saru', 'sari'{]}\end{tabular}} & \begin{tabular}[c]{@{}l@{}} In Gu, there are 3 noun forms.\\ \textit{saru} is a neutral form of the \\adjective \textit{good} and that can \\ not be used with a masculine\\ or a feminine noun, such as \\\textit{seva} (service) is feminine.\\ Similarly \textit{saari} is feminine form. \\ There are also forms like \textit{saras} which\\ can be used with any form of noun.

\end{tabular}                    \\ \hline
\end{tabular}%
}
\caption{Some examples of how translation may affect the AMCG output.}
\label{app:examples}
\end{table*}

% \end{document}
